# Supplementary material for: DropLoss for Long-Tail Instance Segmentation
Source: arXiv:2104.06402 source file (2021-04-17)
Supplement: Supplementary file 1 [file 7_supplimentary.tex]

\section{Overview}

In this supplementary material, we provide additional results to complement the primary manuscript. To further validate our method, we conduct an additional comparison in the no-augmentation setting except horizontal flipping. We also include additional qualitative results. We will make the code for all experiments available online for others to fully reproduce our results.

\section{Data augmentation}

We compare our method against others in an additional setting by removing data augmentation except horizontal flipping. The default data augmentation in the Detectron2 object detection framework \cite{wu2019detectron2} is scale jittering \cite{krizhevsky2012imagenet}, in which the input images are randomly resized to enhance detection of objects at different scales. We include this result for completeness, as the equalization \cite{tan2020eql} baseline did not include scale jittering augmentation in their comparisons \cite{tan2020eql}. Under this additional condition, we find that the DropLoss still achieves the best overall performance as shown in Table \ref{tab:LVIS Effectiveness}.

\begin{table}[th!]
\centering
\caption{\textbf{Results without data augmentation.} Comparison between architecture and backbone settings, evaluated on LVIS v0.5 validation set \cite{GuptaDG19}. We compare BCE (binary cross-entropy), EQL (equalization loss) \cite{tan2020eql} and Drop (DropLoss). AP/AR refers to mask AP/AR, and subscripts `r’, `c’, and `f’ refer to rare, common, and frequent categories. 
\label{tab:LVIS Effectiveness}}
\resizebox{\textwidth}{!}{%
\begin{tabular}{ccccccccccc}
\hline
Architecture & Backbone & Loss & AP (\%) & AP$_\mathrm{50}$ & AP$_\mathrm{75}$ & AP$_\mathrm{r}$ & AP$_\mathrm{c}$ & AP$_\mathrm{f}$ & AR & AP$_\mathrm{bbox}$ \\ \hline
\multirow{3}{*}{Mask R-CNN} & \multirow{3}{*}{R-50-FPN} & BCE & 21.3 & 33.3 & 22.6 & 5.1 & 21.5 & \textbf{27.6} & 28.3 & 21 \\
 &  & EQL & 23.4 & 36.1 & 24.8 & 9.9 & 24.6 & 27.3 & 30.9 & 23 \\
 &  & Drop (Ours) & \textbf{24.3} & \textbf{37.4} & \textbf{25.6} & \textbf{13.1} & \textbf{26.1} & 26.4 & \textbf{33.4} & \textbf{23.9} \\ \hline
\multirow{3}{*}{Mask R-CNN} & \multirow{3}{*}{R-101-FPN} & BCE & 23.6 & 36.6 & 25 & 6 & 25 & \textbf{29} & 31 & 23.4 \\
 &  & EQL & 25.3 & 38.5 & 26.9 & 10.6 & 27.4 & 28.7 & 33.3 & 25.2 \\
 &  & Drop (Ours) & \textbf{26.2} & \textbf{39.7} & \textbf{27.8} & \textbf{14.3} & \textbf{28.8} & 27.6 & \textbf{35.6} & \textbf{26.2} \\ \hline
\end{tabular}%
}
\end{table}

\section{Qualitative results}

Figure \ref{fig:prediction1} and Figure \ref{fig:prediction2} show additional qualitative comparisons of our method against the Mask R-CNN baseline.
Our method consistently recalls more foreground objects due to the rebalancing of discouraging gradients across the category distribution. 
This can be seen in Figure \ref{fig:prediction1} (c-d) where DropLoss more commonly identifies rare category ``pigeon'' as foreground where Mask R-CNN predicts background.
Additionally in Figure \ref{fig:prediction2} (g-h) Mask R-CNN misidentifies common category ``wedding cake'' objects as background or the wrong foreground category despite the objects appearing prominently in the foreground. DropLoss identifies these objects accurately, with several related but inaccurate guesses appearing (``onion'', ``cupcake'', ``whipped cream'').
DropLoss tends towards more fine-grained predictions due to the rebalancing of rare and common categories.
This is evident in Figure \ref{fig:prediction2} (a-b) where DropLoss correctly identifies ``parrot'' where Mask R-CNN predicts coarse-grain frequent category ``bird'', and in Figure \ref{fig:prediction1} (c-d) where DropLoss predicts rare category ``pigeon'' and Mask R-CNN again predicts ``bird''. This example show the bias of Mask R-CNN toward more frequent categories, which may impede fine-grained classification.
Both methods suffer from inaccurate predictions, as can be seen in the challenging examples of Figure \ref{fig:prediction1} (a-b) and Figure \ref{fig:prediction2} (c-d) where both methods suffer from inaccurate foreground and background classifications. However, DropLoss has a consistent advantage in identifying foreground objects.

\begin{figure}
    \subfigure[Mask R-CNN]{%
    \includegraphics[height=0.2\textheight, width=0.49\textwidth]{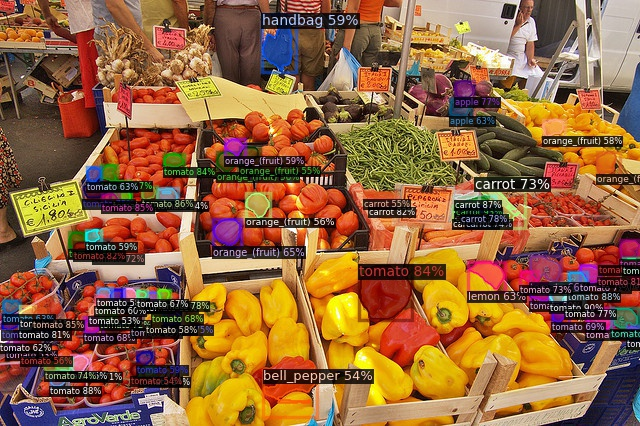}%
    \label{fig:maskrcnn_predict}%
    }\hspace{0cm}
    \subfigure[DropLoss (Ours)]{%
    \includegraphics[height=0.2\textheight, width=0.49\textwidth]{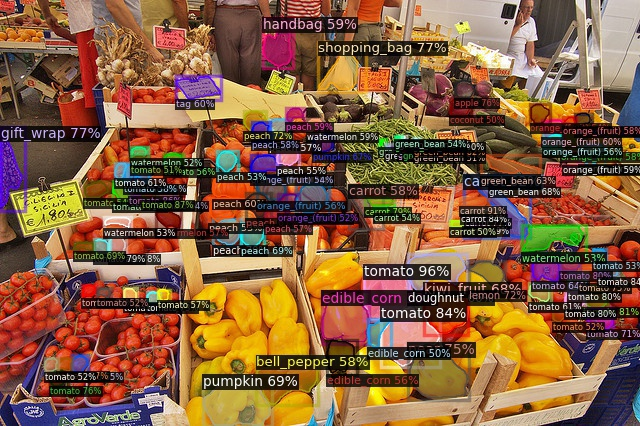}%
    \label{fig:drop_predict}%
    }\hspace{0cm}
    
    \bigskip
    \subfigure[Mask R-CNN]{%
    \includegraphics[height=0.2\textheight, width=0.49\textwidth]{fig/baseline/2.jpg}%
    \label{fig:maskrcnn_predict}%
    }\hspace{0cm}
    \subfigure[DropLoss (Ours)]{%
    \includegraphics[height=0.2\textheight, width=0.49\textwidth]{fig/drop/2.jpg}%
    \label{fig:drop_predict}%
    }\hspace{0cm}
    
    \bigskip
    \subfigure[Mask R-CNN]{%
    \includegraphics[height=0.2\textheight]{fig/baseline/3.jpg}%
    \label{fig:maskrcnn_predict}%
    }\hspace{0cm}
    \subfigure[DropLoss (Ours)]{%
    \includegraphics[height=0.2\textheight]{fig/drop/3.jpg}%
    \label{fig:drop_predict}%
    }\hspace{0cm}
    
    % \bigskip
    % \subfigure[Mask R-CNN]{%
    % \includegraphics[height=0.2\textheight]{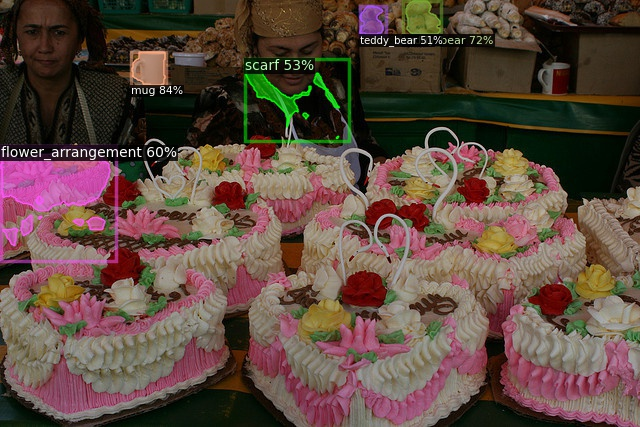}%
    % \label{fig:maskrcnn_predict}%
    % }\hspace{0cm}
    % \subfigure[DropLoss (Ours)]{%
    % \includegraphics[height=0.2\textheight]{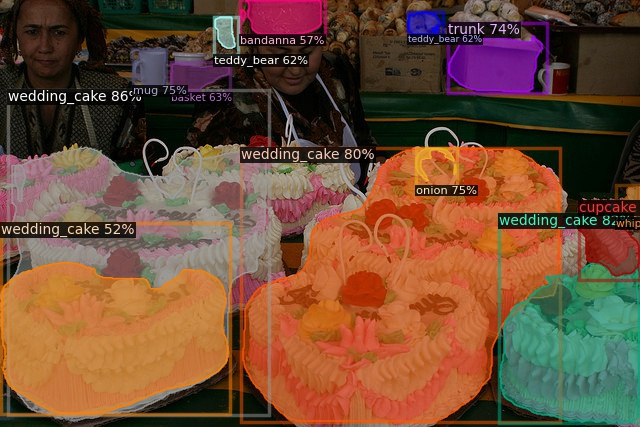}%
    % \label{fig:drop_predict}%
    % }\hspace{0cm}

  \caption{\textbf{Qualitative results.} Visual results of (a,c,e) Mask R-CNN baseline and (b,d,f) the proposed DropLoss. Instances with score > 0.5 are shown. DropLoss adaptively removes background proposal losses of rare and common categories to reduce bias towards misclassifying these objects as background. Rare and common categories pictured include (a)-(b) ``green bean'', ``peach''  (c-d) ``pigeon'', ``bull'', ``tank (storage vessel)'', (e-f) ``gravestone''.}
  \label{fig:prediction1}
\end{figure}

% green bean, peach: rare
% pigeons: rare
% gravestone: common
% wedding cake: common
% calf: common
% bandanna: common
% trunk: common
% basket: frequent
% deer: common
% bull: common
% tank (storage vessel): common
% bird: frequent

\begin{figure}
    \subfigure[Mask R-CNN]{%
    \includegraphics[height=0.2\textheight, width=0.49\textwidth]{fig/baseline/8.jpg}%
    \label{fig:maskrcnn_predict1}%
    }\hspace{0cm}
    \subfigure[DropLoss (Ours)]{%
    \includegraphics[height=0.2\textheight, width=0.49\textwidth]{fig/drop/8.jpg}%
    \label{fig:drop_predict}%
    }\hspace{0cm}
    
    \bigskip
    \subfigure[Mask R-CNN]{%
    \includegraphics[height=0.2\textheight, width=0.49\textwidth]{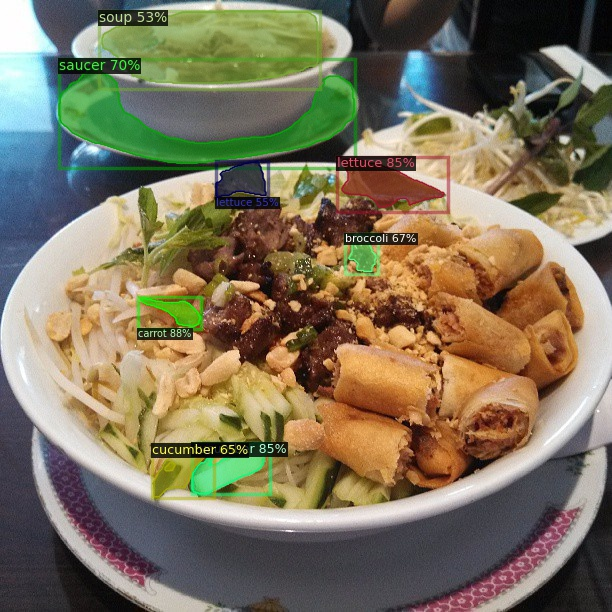}%
    \label{fig:maskrcnn_predict2}%
    }\hspace{0cm}
    \subfigure[DropLoss (Ours)]{%
    \includegraphics[height=0.2\textheight, width=0.49\textwidth]{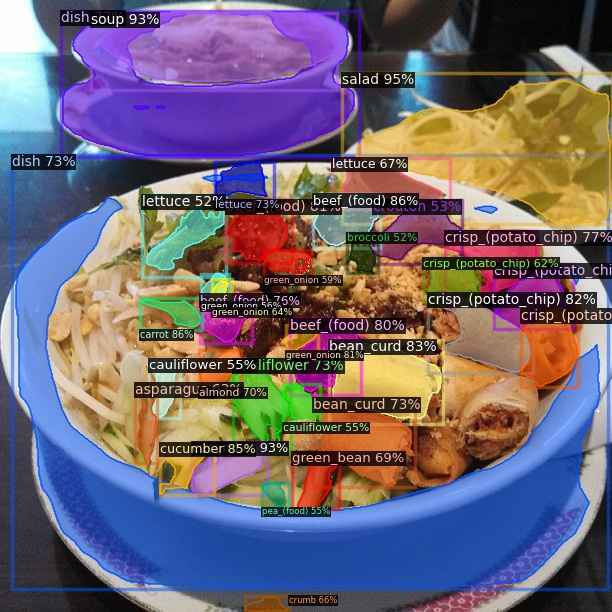}%
    \label{fig:drop_predict}%
    }\hspace{0cm}
    
    \bigskip
    \subfigure[Mask R-CNN]{%
    \includegraphics[height=0.2\textheight, width=0.49\textwidth]{fig/baseline/7.jpg}%
    \label{fig:maskrcnn_predict3}%
    }\hspace{0cm}
    \subfigure[DropLoss (Ours)]{%
    \includegraphics[height=0.2\textheight, width=0.49\textwidth]{fig/drop/7.jpg}%
    \label{fig:drop_predict}%
    }\hspace{0cm}
    
    \bigskip
    \subfigure[Mask R-CNN]{%
    \includegraphics[height=0.2\textheight, width=0.49\textwidth]{fig/baseline/4.jpg}%
    \label{fig:maskrcnn_predict4}%
    }\hspace{0cm}
    \subfigure[DropLoss (Ours)]{%
    \includegraphics[height=0.2\textheight, width=0.49\textwidth]{fig/drop/4.jpg}%
    \label{fig:drop_predict}%
    }\hspace{0cm}

  \caption{\textbf{Qualitative results.} Visual results of (a,c,e,g) Mask R-CNN \cite{he2017mask} baseline and (b,d,f,h) the proposed DropLoss. Instances with score > 0.5 are shown. DropLoss adaptively removes background proposal losses of rare and common categories to reduce bias towards misclassifying these objects as background. Rare and common categories pictured include (a-b) ``parrot'', (c-d) ``beef'', ``crisp (potato chip)'', (e-f) ``pottery'', (g-h) ``wedding cake'', ``bandanna'', ``trunk''.}
  \label{fig:prediction2}
\end{figure}
